# Supplementary material for: Automatic Prompt Selection for Large Language Models
Source: arXiv:2404.02717 source file (2024-04-03)
Supplement: Supplementary file 1 [file appendix.tex]

\subsection{Details of Experiments}

%Toni: to save space, move this to appendix
\subsubsection{The cost of training APS}
A single run of APE requires $\mathcal{O}(p + c \times k \times p)$, where:
\begin{itemize}
    \item p: number of generated prompts
    \item c: number of clusters
    \item k: number of examples per cluster that have ascending distance from the cluster center.
\end{itemize}

This run is to generate training data for preference model. Each generating data task costs between $\$5-10$ with 3000 data samples. The total financial cost for all the experiments $\approx \$30$. Also, it cost more than $\$10$ for evaluation on all the test sets.
